# Supplementary material for: Machine learning accelerated discovery of corrosion-resistant high-entropy alloys
Source: arXiv:2307.06384 ancillary file (2024-01-30)
Supplement: Supplementary file 1 [file si_v3_cz.pdf]

Supporting information

# Machine learning accelerated discovery of corrosion-resistant high-entropy alloys

Cheng Zeng<sup>\*,†</sup>, Andrew Neils, Jack Lesko, Nathan Post<sup>\*</sup>

*The Roux Institute, Northeastern University, Portland, Maine, 04101, United States.*

<sup>†</sup> *The Experiential AI Institute, Northeastern University, Boston, Massachusetts, 02115, United States*

*\* Corresponding authors: Email: c.zeng@northeastern.edu and n.post@northeastern.edu, Tel: +1 401-396-6668 and +1 781-605-8671*

This Supporting Information (SI) includes standard enthalpy of formation for oxides of certain metals, Computational settings of DFT calculations, Details of moment tensor potential (MTP), Random forest classifier for single phase formability, Fast sampling of configurations using the embedded atom method (EAM), First-principles data for MTP, MTP-enabled simulations for corrosion metrics, and Supporting results.

## S-1 Standard enthalpy of formation of oxides

Table S1 summarized the enthalpy of formation of oxides at room temperature (298.15 K). Data are found on NIST Chemistry WebBook. One should note that one mole of  $\text{Cr}_2\text{O}_3$  and  $\text{Al}_2\text{O}_3$  includes two moles of Cr and Al. Therefore, a fair comparison between formation enthalpies of different oxides needs to divide the formation enthalpy by the number of metal element.

## S-2 Computational settings for DFT calculations

Grid-based projector-augmented wave code (GPAW) was used for all DFT calculations [1]. The Generalized Gradient Approximation (GGA) exchange-correlation functional parameterized by

**Table S1:** Molar enthalpy of oxide formation for Al, Cr, Fe, Co and Ni. Data are excerpted from [NIST Chemistry Webbook](#).

| Oxide                   | $\Delta_f H_{\text{solid}}^0$ [kJ/mol] |
|-------------------------|----------------------------------------|
| $\text{Al}_2\text{O}_3$ | -1675.7                                |
| $\text{Cr}_2\text{O}_3$ | -1134.70                               |
| FeO                     | -272.04                                |
| CoO                     | -237.74                                |
| NiO                     | -239.7                                 |

Perdew-Burke-Ernzerhof (PBE) was used with a plane wave cutoff of 350 eV [2]. Fermi-Dirac smearing of 0.1 eV was employed for fast convergence, and the energetics were extrapolated to 0 K. All calculations were performed including spin polarization. To sample the Brillouin zone, the number of k points for any dimension is set by a floor function  $\lfloor 30/l \rfloor$  where  $l$  is the length of the dimension. For surface structures, a dipole correction was applied in the direction normal to the surface. Convergence of self-consistent field (SCF) calculations were achieved when the energy difference between the last three steps is less than 0.0001 eV/electron.

### S-3 Details of momentum tensor potentials

In spirit to finite-ranged machine learning potentials, momentum tensor potential (MTP) defines the total energy  $E$  as the sum of contributions of local chemical environments ( $V(\mathbf{n}_i)$ ). The atomic local contribution  $V(\mathbf{n}_i)$  is expanded by a linear combination of basis functions. Each of the basis function is a contraction of moment tensor descriptors to yield scalars. The moment comprises of two components—one component is a radial function to control the finite-ranged two-body interactions, and the other component is tensor of a certain rank encoding angular information of the atomic environment. By definition, the as-built basis functions preserve the rotation, permutation and reflection symmetries. The maximum level of contraction ( $\text{lev}_{\text{max}}$ ) allowed defines the functional form of MTP. For high-entropy alloy AlCrFeCoNi, we used  $\text{lev}_{\text{max}}=20$  with Chebyshev polynomials as the radial basis functions. The minimum and cutoff distances of interactions were set as 2 and 5 Å, respectively. For five-species materials with  $\text{lev}_{\text{max}}=20$ , the total number of parameters to be fitted is 1293. For the breakdown of the number of parameters, readers should consult the work by Novikov et al. [3].

### S-4 Random forest classifier for single phase formability

#### Description of features

As mentioned, we built eight features on top of a given chemical composition. Those features consist of atomic size difference ( $\delta$ ), mixing entropy ( $\Delta S_{\text{mix}}$ ), mixing enthalpy ( $\Delta H_{\text{mix}}$ ), Pauli electronegativity difference ( $\Delta\chi$ ), molar volume ( $V_m$ ), bulk modulus ( $K$ ), melting temperature ( $T_m$ ), and valence electron concentration (VEC). For the last four features, they are obtained by taking the composition-weighted average of the corresponding atomic attributes. The mixing entropy is defined as  $\Delta S_{\text{mix}} = -R \sum_{i=1}^n c_i \ln(c_i)$ , where  $R$  is the ideal gas constant and  $c_i$  is the composition of element  $i$ . The Pauli electronegativity difference is expressed as  $\Delta\chi = \sqrt{\sum_i c_i (\chi_i - \bar{\chi})^2}$ , where  $\chi_i$  and  $\bar{\chi}$  are respective electronegativity of element  $i$  and the composition-weighted average of electronegativity. The size difference is given by  $\delta = 100 \times \sqrt{\sum_i c_i (1 - \frac{r_i}{\bar{r}})^2}$  where  $r_i$  and  $\bar{r}$  represent the size of atom  $i$  and the weighted average of atom sizes, respectively. The mixing enthalpy reads as  $\Delta H_{\text{mix}} = 4 \sum_{i=1}^n \sum_{j>i}^n H_{ij} c_i c_j$ , where the binary interaction term is calculated based on the Miedema model [4].

The size, melting temperature, valence electron concentration and molar volume of each element are retrieved from the ‘[mendeleeev](#)’ python package. The bulk modulus of each element is excerpted from the plot on [the website for periodic table](#) using [WebPlotDigitizer](#). For some missing

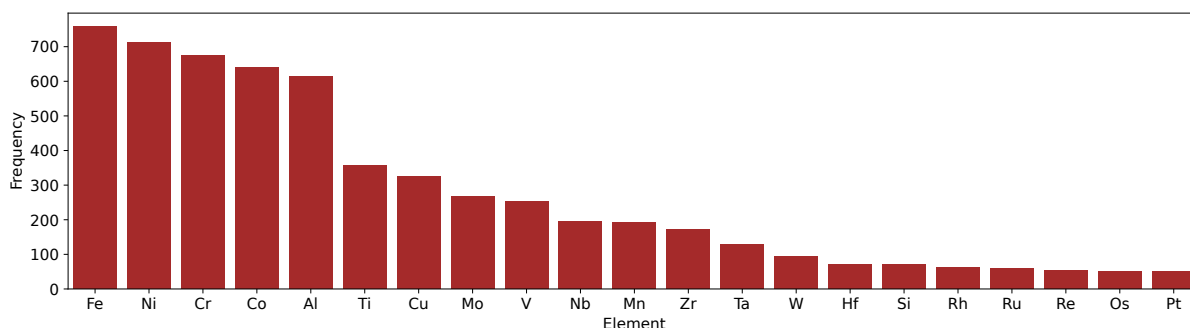

**Figure S1:** Frequency of elements in the experimental dataset.

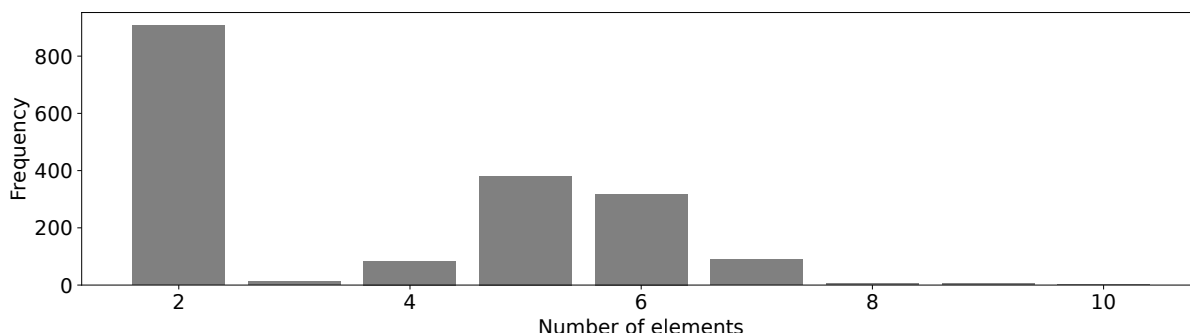

**Figure S2:** Frequency of number of elements in the experimental data.

bulk modulus and electronegativity values, web values were used. The Midema model calculations were carried out using ‘[qmpy](#)’ python package.

## Exploratory data analysis

Figure S1 shows the frequency of elements found in the experimental data. It is clear that the most commonly used five elements are Fe, Ni, Cr, Co and Al, and those noble metals such as Pt and Au are barely used.

Figure S2 summarizes the number of elements for each alloy in the experimental dataset. Most of the alloys are binary and most high-entropy alloys are with five or six elements.

Figure S3 shows the class-wise distribution of values for each feature. A glimpse of these box plots indicate that there are no strong linear dependence of single phase formability with any specific features, implying that non-linear models are needed to describe the complex interactions between feature and output labels.

## Model parameters

We built the random forest model using scikit-learn python package (<https://scikit-learn.org/stable/>). We set the number of estimators (decision trees), max depth of each estimator, minimum samples to be split as 100, 20 and 4, respectively. A ‘minmax’ scaler was utilized to scale feature values to the range between -1 and 1 because all feature values are well bounded.

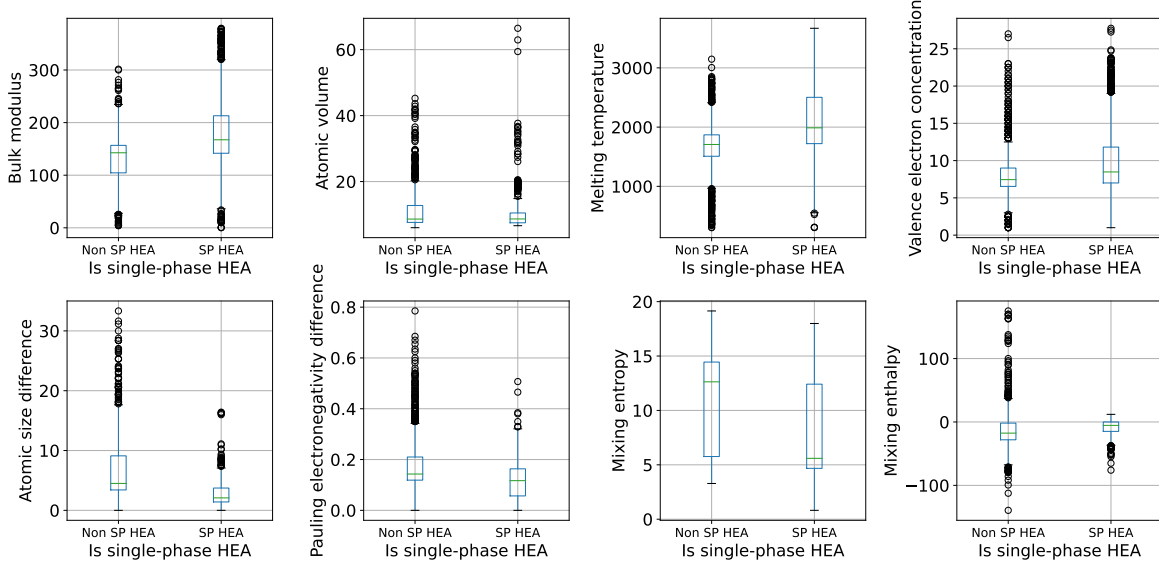

**Figure S3:** Class-specific feature value distributions.

## S-5 Fast sampling of configurations using EAM

To facilitate the process of generation of training structures, we first created bulk FCC structures with a supercell of  $3 \times 3 \times 3$  (108 atoms) for  $\text{Al}_x(\text{CrFeCoNi})_{100-x}$  with Al compositions being 0, 5, 10, 15 and 20%. The atoms in the supercell were randomly distributed. We performed relaxation using LAMMPS to optimize the lattice geometry and atomic positions at the same time. For the relaxation trajectory of each Al composition, we chose the structures at every 10th relaxation step to be evaluated by first-principles calculations. In total, 150 bulk structures chosen from relaxation were calculated. Starting with the relaxed structures, we performed NVT molecular dynamic (MD) simulations using Langevin dynamics at a temperature of 1700 K, a friction coefficient of 0.002 and time step of 5 fs. 5000 MD steps were carried out and 100 images for each Al composition were saved, out of which 20 structures were further selected using a farthest point sampling algorithm. 20 structures were selected for each Al composition for the purpose of efficiency of first-principles calculations as well as for preserving most statistical info held by the original 100 structures. Those 20 structures were reevaluated by First-principles calculations. Moreover, we performed Markov chain Monte-Carlo (MCMC) simulations to sample more diverse structures. MC simulations were performed with canonical ensemble at a temperature of 500 K. At each MC step, two neighboring atoms with different types are exchanged and a new structure is created. We aimed to sample more possible local minima using MCMC simulations. The new structure is accepted if the potential energy drops; otherwise, it will be accepted with a Boltzmann probability if the potential energy increases. Numbers of MC steps were chosen to ensure that on average at least 40 times of swap were performed for each atom in the system. For each Al composition, 50 MC structures were randomly selected for DFT evaluation. The MD and MC simulations were conducted with Atomic Simulation Environment (ASE) [5] and using the ASE-MTP interface available at [ASEMTP](#). For FCC(111) surfaces, atomic structures with a supercell of  $5 \times 5 \times 5$  were created for each Al composition. The same procedure as the sampling for bulk structures was carried out to sample diverse

**Table S2:** Breakdown of the training data.

| Data type           | # training data | # atoms |
|---------------------|-----------------|---------|
| Bulk, relaxation    | 150             | 108     |
| Bulk, MD            | 99              | 108     |
| Bulk, MCMC          | 242             | 108     |
| Bulk, simple        | 365             | 1–54    |
| Surface, relaxation | 234             | 125     |
| Surface, MD         | 99              | 125     |
| Surface, MCMC       | 242             | 125     |
| Surface, simple     | 138             | 5, 16   |
| Total               | 1569            | NA      |

**Table S3:** Breakdown of ‘simple’ structures. SQS is short for special quasi-random structures.

| Data type                           | # training data | # atoms             |
|-------------------------------------|-----------------|---------------------|
| Bulk, simple, SQS                   | 120             | 24, 25, 27          |
| Bulk, simple, unary and binary      | 245             | 1, 2, 4, 27, 32, 54 |
| Surface, simple, 1x1x5 surface cell | 108             | 5                   |
| Surface, simple, 2x2x4 surface cell | 30              | 16                  |

surface structures.

## S-6 First-principles data used to construct MTP

We carried out first-principles calculations to refine the properties (energy and forces) of the structures sampled using EAM. Together with the simple bulk structures and surface structures with numbers of elements from one to five, in total 1569 first-principles data were curated. Numbers of training data per simulation task were given in Table S2. Numbers of training data for ‘simple’ structures were listed in Table S3. Note that the number of structures shown in the table may be different from that sent to DFT calculations because some of those calculations did not converge. The relaxation, MD and MCMC structures have been elaborated in the above section. The simple bulk structures include first-principles relaxation trajectories for ternary, quaternary and quinary special quasi-random structures generated with alloy ATAT, and relaxation trajectories for simple bulk structures with no more than two elements. The simple surface structures include five-atom FCC111 5-layer  $1 \times 1$  surfaces with one to five elements and 16-atom one-element FCC111 surface structures. High-throughput DFT calculations were operated using methods developed in our previous work [6].

## S-7 MTP-enabled simulations used to calculate corrosion metrics

To obtain the results shown in Figure 2, for each Al composition of  $\text{Al}_x(\text{CrFeCoNi})_{100-x}$ , we create FCC\_A1 and  $\text{L1}_2$  structures using a supercell of  $5 \times 5 \times 5$  (500 atoms), and B2 structures using a supercell of  $7 \times 7 \times 7$ . We then optimized those structures in ASE using a force stopping criterion of 0.05 eV/Å. As the number of atoms for FCC and BCC structures are different, we cannot directly compare the total energies. Instead, we compare the cohesive energies as shown in Figure 2.

To obtain the values of  $PBR_{\text{Cr}}$  as shown in Figure 3(b), we created  $\text{L1}_2$  structures with systematically varied Al and Cr compositions for  $\text{Al}_x\text{Cr}_y(\text{FeCoNi})_{100-x-y}$  using a composition interval of 5%. We performed the structure optimization to find the stable lattice cell and atomic positions. We found linear dependences of lattice constants with both Al and Cr compositions. The fitted coefficients for Al and Cr compositions are respectively 3.26672181e-03 and 6.81928982e-05, respectively, suggesting a stronger dependence on Al compositions. Therefore, for any pair of Al and Cr for  $\text{Al}_x\text{Cr}_y(\text{FeCoNi})_{100-x-y}$ , we can find the geometry, hence the volume of Cr element in the alloys. The volume of Cr will be used to calculate  $PBR_{\text{Cr}}$ .

In order to calculate the surface energies as shown in Figure 3(c), the bulk systems involved are the  $\text{L1}_2$  structures used for  $PBR_{\text{Cr}}$  while for the surface structures, we created a  $20 \times 20 \times 5$  (2000 atoms) surface cell to ensure that the periodicity in the surface directions will not affect the arrangement of atoms. We performed MCMC simulations with around 80000 MC steps and a temperature of 500 K to identify stable structures. The surface energies were calculated by taking the difference between energies of surface systems and bulk systems, following by a division over the surface area.

## S-8 Supporting results

### Feature importance for random forest classifiers

With the random forest classifier, we analyzed the importance of all features using shapley values. The results are plotted in Figure S4. The most important two features are mixing entropy and atomic size difference. The importance of mixing entropy is twofold and competitive. On one hand, thermodynamically high entropy will encourage the system to be well mixed to reduce the Gibbs free energy. On the other hand, mixing more elements tend to be more difficult because there is larger chance attributes among some elements can be highly varied. The importance of atomic size difference is in alignment with intuition that mixing elements with different sizes is more challenging. Interestingly, the least important feature is valence electron concentration although VEC can be good indicator of which type of single phase structures will be formed [7].

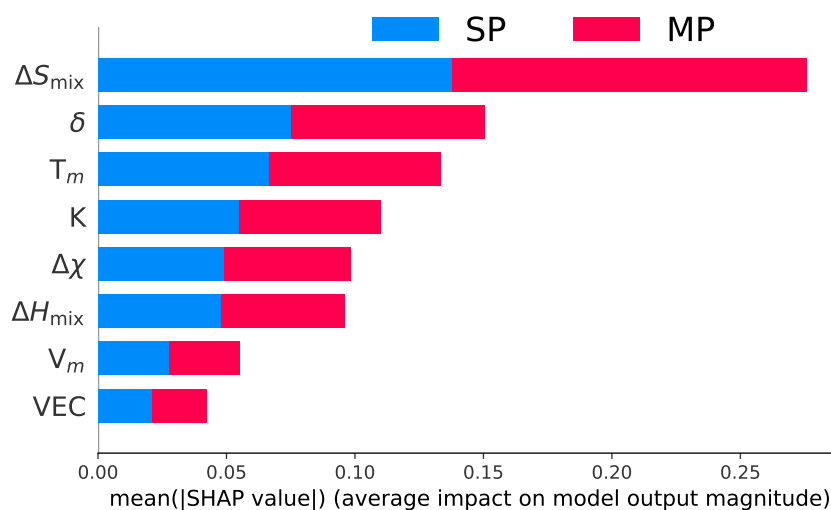

**Figure S4:** Class-specific shapley feature importance for the trained random forest classifier. SP and MP represent single phase and multiple phase, respectively.

## References

- [1] Dohn, A.O.; Jónsson, E.Ö.; Levi, G.; Mortensen, J.J.; Lopez-Acevedo, O.; Thygesen, K.S.; Jacobsen, K.W.; Ulstrup, J.; Henriksen, N.E.; Møller, K.B.; Jónsson, H. Grid-Based Projector Augmented Wave (GPAW) Implementation of Quantum Mechanics/Molecular Mechanics (QM/MM) Electrostatic Embedding and Application to a Solvated Diplatinum Complex. *Journal of Chemical Theory and Computation* **2017**; 13, 6010–6022.
- [2] Perdew, J.P.; Burke, K.; Ernzerhof, M. Generalized Gradient Approximation Made Simple. *Physical Review Letters* **1996**; 77, 3865–3868.
- [3] Novikov, I.S.; Gubaev, K.; Podryabinkin, E.V.; Shapeev, A.V. The MLIP package: moment tensor potentials with MPI and active learning. *Mach. Learn.: Sci. Technol.* **2020**; 2, 025002. Publisher: IOP Publishing.
- [4] Zhang, R.F.; Zhang, S.H.; He, Z.J.; Jing, J.; Sheng, S.H. Miedema Calculator: A thermodynamic platform for predicting formation enthalpies of alloys within framework of Miedema's Theory. *Computer Physics Communications* **2016**; 209, 58–69.
- [5] Hjorth Larsen, A.; Jørgen Mortensen, J.; Blomqvist, J.; Castelli, I.E.; Christensen, R.; Dułak, M.; Friis, J.; Groves, M.N.; Hammer, B.; Hargus, C.; Hermes, E.D.; Jennings, P.C.; Bjerre Jensen, P.; Kermode, J.; Kitchin, J.R.; Leonhard Kolsbjerg, E.; Kubal, J.; Kaasbjerg, K.; Lysgaard, S.; Bergmann Maronsson, J.; Maxson, T.; Olsen, T.; Pastewka, L.; Peterson, A.; Rostgaard, C.; Schiøtz, J.; Schütt, O.; Strange, M.; Thygesen, K.S.; Vegge, T.; Vilhelmsen, L.; Walter, M.; Zeng, Z.; Jacobsen, K.W. The atomic simulation environment—a Python library for working with atoms. *Journal of Physics: Condensed Matter* **2017**; 29, 273002.

- [6] Zeng, C.; Chen, X.; Peterson, A.A. A nearsighted force-training approach to systematically generate training data for the machine learning of large atomic structures. *The Journal of Chemical Physics* **2022**; 156, 064104.
- [7] Steurer, W. Single-phase high-entropy alloys – A critical update. *Materials Characterization* **2020**; 162, 110179.
